# Supplementary material for: FMI: Fast and Cheap Message Passing for Serverless Functions
Source: arXiv:2305.08763 source file (2023-05-15)
Supplement: Supplementary file 1 [file appendix.tex]

HOLE PUNCHING:
The technique depends on the internal implementation of the gateway~\cite{rfc3489}.
In a \emph{full cone NAT}, the internal source address of a four-tuple is always
replaced by the same external address.
Any other party can use use this external address to communicate with the
internal system that initiated the connection.
However, a \emph{symmetric NAT} employs different tuple translations for
different destinations.
There, a message sent to a peer behind the gateway is successful only when the
message originated from the corresponding destination.
There, no hole punching is possible.
Furthermore, \emph{restricted cone NAT} adds to a full cone solution the
requirement that packets from an external party are forwarded if and only if
the party behind NAT has sent messages before to this external peer.
Both peers need to initiate connections repeatedly, and it is undefined whose
connection request will ultimately succeed.

COLLECTIVES:

In MPI, \textbf{System optimizations} provide multi-protocol approaches to benefit from
intra-node communication~\cite{1437304,10.1145/2462902.2462903,10.5555/3291656.3291695,6047221,10.1007/11557265_11},
including thread-based runtimes for faster synchronization~\cite{10.1145/2462902.2462903,10.1145/2442516.2442534,6877451,10.1145/3339186.3339199}.
FaaS functions however are often co-located on the same machine, but sandbox virtualization prevents fast and
assisted local communication.

MPI collectives are specialized for \textbf{network transport} protocols~\cite{PATARASUK2009117,10.1145/301104.301116,8457871,10.5555/2396095.2396108},
including remote memory access (RMA)~\cite{10.1007/11602569_19} and
accelerators~\cite{10.1145/3208040.3208054,10.1145/3236367.3236381,nvidiaNCCL}.
Serverless heterogeneity is increasing with RMA~\cite{copik2021rfaas} and GPUs~\cite{satzke2020efficient,kim2018gpu},
but abstractions of collective operations are needed to ensure high performance and portability.

Collective algorithms can be tuned to specific \textbf{network topology}~\cite{9229573,PJESIVACGRBOVIC2007613,1592716,10.1145/2145816.2145823,846009}.
The ephemeral functions should consider mapping task layout to the dynamically
changing topology of workers~\cite{7530080,6468466,10.1145/3127024.3127031}.
Furthermore, collectives are optimized for specific needs of \textbf{applications},
such as bandwidth and sparsity optimizations in machine learning~\cite{10.1145/3126908.3126954,10.1145/2966884.2966912,10.1145/3295500.3356222,8514855},
non-blocking communication~\cite{5160935,5348811},
and varying compute--to--communication ratio~\cite{9477174}.
Finally, the performance of collectives can be sensitive to imbalance and noise~\cite{faraj2008study,10.1145/3208040.3208054}
and require dynamic adaptive schemes for robustness~\cite{faraj2008study,4536308}.
This is a significant problem in serverless, where performance variability is high~\cite{copik2021sebs}.

Simpler last point:

Finally, the performance of collectives can be sensitive to imbalance and noise~\cite{faraj2008study,10.1145/3208040.3208054}
and require dynamic adaptive schemes for robustness~\cite{faraj2008study,4536308} -- this is no different in serverless, where performance variability is high~\cite{copik2021sebs}.
